# Supplementary material for: ForceHarness: Turning Force into Action and Physics for Frozen Frontier Models
Source: arXiv:2611.21099 source file (2026-11-16)
Supplement: Supplementary file 1 [file 0_setup.tex]

\makeatletter
\providecommand{\FloatBarrier}{\par\begingroup\let\@elt\relax
  \edef\@tempa{\@deferlist\@dbldeferlist}\def\@tempb{}%
  \ifx\@tempa\@tempb\endgroup\else\endgroup\clearpage\fi}
\makeatother

\counterwithin{figure}{section}
\counterwithin{table}{section}
\counterwithin{equation}{section}
\renewcommand{\thefigure}{\thesection\arabic{figure}}
\renewcommand{\thetable}{\thesection\arabic{table}}
\renewcommand{\theequation}{\thesection\arabic{equation}}
\makeatletter
\@ifundefined{theHfigure}{}{%
  \renewcommand{\theHfigure}{supp.\thefigure}%
  \renewcommand{\theHtable}{supp.\thetable}%
  \renewcommand{\theHequation}{supp.\theequation}}
\makeatother

\newcommand{\code}[1]{\textit{#1}}

\definecolor{fhnavy}{HTML}{1E467A}
\definecolor{fhteal}{HTML}{1E7F76}
\definecolor{fhgrey}{HTML}{6B7280}
\definecolor{fhrule}{HTML}{9AA3B2}

\newcounter{pcline}
\newlength{\pcind}\setlength{\pcind}{0.85em}
\newcommand{\Kw}[1]{\textbf{#1}}
\newcommand{\Cm}[1]{{\color{fhgrey}\textit{#1}}}
\newcommand{\Fq}[1]{{\color{fhteal}#1}}
\newcommand{\Tq}[1]{{\color{fhnavy}#1}}
\newcommand{\Fn}[1]{\textsc{#1}}
\newcommand{\PL}[2]{\par\noindent\stepcounter{pcline}%
  \makebox[1.1em][r]{\color{fhgrey}\tiny\arabic{pcline}}\hspace{0.45em}\hspace{#1\pcind}%
  \parbox[t]{\dimexpr\linewidth-1.55em-#1\pcind\relax}{\raggedright\strut#2\strut}}
\newenvironment{pcode}[1]{%
  \setcounter{pcline}{0}\scriptsize\setlength{\parskip}{0pt}%
  \par\noindent\textbf{#1}\par\nointerlineskip\vspace{2.2pt}%
  \noindent{\color{fhrule}\rule{\linewidth}{0.5pt}}\par\vspace{0.8pt}}%
 {\par\vspace{1.2pt}\noindent{\color{fhrule}\rule{\linewidth}{0.5pt}}\par}
\newlength{\cardgfx}\setlength{\cardgfx}{0.292\textwidth}
\newlength{\cardcode}\setlength{\cardcode}{0.372\textwidth}
\newlength{\tcardw}\setlength{\tcardw}{0.488\textwidth}
\newlength{\tcardimg}\setlength{\tcardimg}{0.385\tcardw}
\newcommand{\TCl}[1]{\par\hangindent=0.7em\hangafter=1\noindent{\color{fhnavy}\textbf{#1}}\enspace}
\newcommand{\TaskCard}[7]{%
  \begin{minipage}[t]{\tcardw}\vspace{0pt}%
  \begin{minipage}[t]{\tcardimg}\vspace{0pt}%
    {\setlength{\fboxsep}{0pt}\setlength{\fboxrule}{0.4pt}\color{fhrule}\fbox{\includegraphics[width=\dimexpr\linewidth-0.8pt\relax]{#1}}}%
  \end{minipage}\hfill
  \begin{minipage}[t]{\dimexpr\tcardw-\tcardimg-0.8em\relax}\vspace{-1pt}\scriptsize\raggedright
    {\footnotesize\bfseries #2}\enspace{\color{fhgrey}\itshape #3}\vspace{1pt}%
    \TCl{Hidden}#4\TCl{Told}#5\TCl{Success}#6\TCl{Expert}#7\par
  \end{minipage}%
  \end{minipage}}
\newcommand{\TaskNote}[2]{%
  \begin{minipage}[t]{\tcardw}\vspace{0pt}%
  {\setlength{\fboxsep}{5pt}\colorbox{fhrule!14}{\begin{minipage}[t]{\dimexpr\tcardw-10pt\relax}\scriptsize\raggedright
    {\footnotesize\bfseries #1}\par\vspace{2pt}#2\end{minipage}}}%
  \end{minipage}}
\newcommand{\fixedtable}[1]{\renewcommand{\thetable}{#1}\renewcommand{\theHtable}{supp.#1}}
\newcommand{\fixedfigure}[1]{\renewcommand{\thefigure}{#1}\renewcommand{\theHfigure}{supp.#1}}
\renewcommand{\topfraction}{0.9}
\renewcommand{\dbltopfraction}{0.9}
\renewcommand{\bottomfraction}{0.6}
\renewcommand{\textfraction}{0.08}
\renewcommand{\floatpagefraction}{0.85}
\renewcommand{\dblfloatpagefraction}{0.85}
\setcounter{topnumber}{4}
\setcounter{dbltopnumber}{4}
\setcounter{totalnumber}{6}
